# Supplementary material for: Direct extraction of excitation energies from ensemble density-functional theory
Source: arXiv:1703.10738 source file (2017-06-29)
Supplement: Supplementary file 1 [file supplemental.pdf]

# Supplemental material for "Direct extraction of excitation energies from ensemble density-functional theory"

Zeng-hui Yang,[1] Aurora Pribram-Jones,[2,3] Kieron Burke,[4] and Carsten A. Ullrich[5]

[1] *Microsystem and Terahertz Research Center, China Academy of Engineering Physics, Chengdu, China 610200*
[2] *Department of Chemistry, University of California, Berkeley, CA 94720, USA*
[3] *Lawrence Livermore National Laboratory, Livermore CA 94550, USA*
[4] *Department of Chemistry, University of California-Irvine, Irvine, CA 92697, USA*
[5] *Department of Physics and Astronomy, University of Missouri, Columbia, MO 65211, USA*

(Dated: May 26, 2017)

This supplemental material contains the detailed derivation of the direct ensemble correction (DEC), the calculation details for DEC/SEHX and numerically exact DEC, examples showing the sensitivity of both DEC and time-dependent density-functional theory to the quality of the Kohn-Sham ground state, and additional atomic and ionic calculation results calculated using DEC/SEHX.

## DETAILS OF THE DERIVATION

### The GOK ensemble

In the main text, we write the ensembles and ensemble energies in terms of multiplets. Here we write them in terms of the individual states for clarity and consistency with the structure of the SEHX approximation.

The GOK ensemble is defined by

$$\mathtt{w}_{i,k} = \begin{cases} \frac{1-\mathtt{w}g_I}{M_I - g_I} & i < I, \\ \mathtt{w} & i = I, \end{cases} \tag{1}$$

where $k$ denotes the individual states in the multiplet $i$.

The density matrix of the GOK ensemble is

$$\hat{D}_{I,\mathtt{w}} = \frac{1-\mathtt{w}g_I}{M_{I-1}} \sum_{i=0}^{I-1} \hat{P}_i + \mathtt{w}\hat{P}_I, \tag{2}$$

where $\hat{P}_i = \sum_{k=1}^{g_i} |i,k\rangle\langle i,k|$, and $k$ sums over the degenerate states of the $i$th multiplet. With the density matrix known, one obtains the corresponding ensemble density and energy:

$$\begin{aligned} n_{I,\mathtt{w}}(\mathbf{r}) &= \mathrm{tr}\{\hat{D}_{I,\mathtt{w}}\hat{n}(\mathbf{r})\} \\ &= \frac{1-\mathtt{w}g_I}{M_{I-1}} \sum_{i=0}^{I-1} \mathrm{tr}\{\hat{P}_i\hat{n}(\mathbf{r})\} \\ &\quad + \mathtt{w}\,\mathrm{tr}\{\hat{P}_I\hat{n}(\mathbf{r})\}, \end{aligned} \tag{3}$$

and

$$\begin{aligned} E_{I,\mathtt{w}} &= \mathrm{tr}\{\hat{D}_{I,\mathtt{w}}\hat{H}\} \\ &= \frac{1-\mathtt{w}g_I}{M_{I-1}} \sum_{i=0}^{I-1} g_i\bar{E}_i + \mathtt{w}g_I\bar{E}_I, \end{aligned} \tag{4}$$

where $\bar{E}_i$ is the energy of the $i$th multiplet. By differentiating Eq. (4) with respect to $\mathtt{w}$, one obtains an equation for the excitation energy $\omega_I = \bar{E}_I - \bar{E}_0$ [1]

$$\omega_I = \frac{1}{g_I} \left.\frac{dE_{I,\mathtt{w}}}{d\mathtt{w}}\right|_{\mathtt{w}=\mathtt{w}_I} + \sum_{i=1}^{I-1} \frac{1}{M_i} \left.\frac{dE_{i,\mathtt{w}}}{d\mathtt{w}}\right|_{\mathtt{w}=\mathtt{w}_i}, \tag{5}$$

where $E_{i,\mathtt{w}}$ is the ensemble energy of an ensemble with the $i$th multiplet as its highest state, and $\mathtt{w}_i$ is any valid weight satisfying $\mathtt{w}_i \in [0, 1/M_i]$. According to Eq. (5), a calculation of the $I$th multiplet excitation energy also requires calculations of all the lower ensembles.

Equation (5) requires $dE_{I,\mathtt{w}}/d\mathtt{w}$, which is derived in Ref. [1], and here we write the derivation in the following. The ensemble energy $E_{I,\mathtt{w}}$ is a functional of the ensemble density, which is reproduced by the non-interacting ensemble Kohn-Sham system. The functional is

$$\begin{aligned} E_{I,\mathtt{w}}[n] =& T_{\mathrm{s},I,\mathtt{w}}[n] + \int d^3r\; n(\mathbf{r}) v_{\mathrm{ext}}(\mathbf{r}) \\ &+ \frac{1}{2} \int\int d^3r d^3r'\; \frac{n(\mathbf{r})n(\mathbf{r}')}{|\mathbf{r}-\mathbf{r}'|} + E_{\mathrm{xc},I,\mathtt{w}}[n]. \end{aligned} \tag{6}$$

The non-interacting kinetic energy can be written as

$$\begin{aligned} T_{\mathrm{s},I,\mathtt{w}}[n] =& -\int d^3r\; n_{I,\mathtt{w}}(\mathbf{r}) v_{\mathrm{s},I,\mathtt{w}}(\mathbf{r}) \\ &+ \sum_{\mu=0}^{\infty} \left( \frac{1-\mathtt{w}g_I}{M_{I-1}} \sum_{i=0}^{I-1}\sum_{k=1}^{g_i} f_{i,k,\mu} + \mathtt{w}\sum_{k=1}^{g_I} f_{I,k,\mu} \right) \epsilon_\mu^I, \end{aligned} \tag{7}$$

where $v_{\mathrm{s},I,\mathtt{w}}$ is the ensemble Kohn-Sham (KS) potential, $j$ sums over all the ensemble Kohn-Sham orbitals, $\epsilon_\mu^I$ is the ensemble Kohn-Sham orbital energy (depends on both $n$ and $w$), $f_{i,k,\mu}$ is the occupation number of the $\mu$-th orbital in the $k$-th Kohn-Sham wavefunction of the $i$-th multiplet, which is a Slater determinant in Ref. [1]. With Eqs. (6) and (7), following the derivation of Ref. [1]'s Eqs. (31) to (34), one obtains

$$\begin{aligned} \frac{dE_{I,\mathtt{w}}}{d\mathtt{w}} =& \sum_{\mu=0}^{\infty} \left( \sum_{k=1}^{g_I} f_{I,k,\mu} - \frac{g_I}{M_{I-1}} \sum_{i=0}^{I-1}\sum_{k=1}^{g_i} f_{i,k,\mu} \right) \epsilon_\mu^I \\ &+ \left.\frac{\partial E_{\mathrm{xc},I,\mathtt{w}}[n]}{\partial \mathtt{w}}\right|_{n=n_{I,\mathtt{w}}}, \end{aligned} \tag{8}$$

as shown in Ref. [1]. Inserting Eq. (8) into Eq. (5) yields the full formula for calculating the excitation energy using the GOK ensemble.

We do not include in Eq. (8) symmetrizations introduced later in Eq. (13), since such an equation is not used in this work. There is no difficulty in considering symmetrizations in the derivation, however.

### The GOKII ensemble

For the GOKII ensemble defined by

$$\mathtt{w}_{i,k} = \begin{cases} \frac{1-\mathtt{w}(M_I - g_0)}{g_0} & i = 0, \\ \mathtt{w} & i > 0, \end{cases} \tag{9}$$

the density matrix, ensemble density, and ensemble energy are

$$\hat{D}^{\rm GOKII}_{I,\mathtt{w}} = \frac{1-\mathtt{w}(M_I - g_0)}{g_0}\hat{P}_0 + \mathtt{w}\sum_{i=1}^{I}\hat{P}_i, \tag{10}$$

$$\begin{aligned} n^{\rm GOKII}_{I,\mathtt{w}}(\mathbf{r}) &= {\rm tr}\{\hat{D}^{\rm GOKII}_{I,\mathtt{w}}\hat{n}(\mathbf{r})\} \\ &= \frac{1-\mathtt{w}(M_I - g_0)}{g_0}{\rm tr}\{\hat{P}_0\hat{n}(\mathbf{r})\} \\ &\quad + \mathtt{w}\sum_{i=1}^{I}{\rm tr}\{\hat{P}_i\hat{n}(\mathbf{r})\}, \end{aligned} \tag{11}$$

and

$$\begin{aligned} E^{\rm GOKII}_{I,\mathtt{w}} &= {\rm tr}\{\hat{D}^{\rm GOKII}_{I,\mathtt{w}}\hat{H}\} \\ &= [1-\mathtt{w}(M_I - g_0)]]\bar{E}_0 + \mathtt{w}\sum_{i=1}^{I} g_i\bar{E}_I. \end{aligned} \tag{12}$$

Our previous work [2, 3] demonstrates that the KS excited-state wavefunctions $|i,k\rangle$ should be linear combinations of degenerate KS Slater determinants, so that they would have the same spatial and spin symmetry as the actual excited states:

$$\Phi_{i,k}(\mathbf{r}_1\ldots\mathbf{r}_N) = \sum_{p=1}^{\tilde{g}_{\tilde{i}}} C_{i,k,p}\tilde{\Phi}_{\tilde{i},p}(\mathbf{r}_1\ldots\mathbf{r}_N), \tag{13}$$

where $\tilde{g}_{\tilde{i}}$ is the number of degenerate KS Slater determinants corresponding to the actual multiplet $i$ (and KS multiplet $\tilde{i}$), $\tilde{\Phi}_{\tilde{i},p}$ is the $p$-th KS Slater determinant belonging to the KS multiplet $\tilde{i}$, and $C_{i,k,p}$ are the mixing coefficients satisfying $\sum_{p=1}^{\tilde{g}_{\tilde{i}}} |C_{i,k,p}|^2 = 1$. As an example of the difference between $g_i$ and $\tilde{g}_{\tilde{i}}$, consider the first and second excited states of the helium atom: the first excited state is a triplet and the second is a singlet, so $g_1 = 3$ and $g_2 = 1$; but for the KS system there are 4 degenerate Slater determinants, so $\tilde{g}_{\tilde{1}} = 4$. $\tilde{g}_{\tilde{2}}$ is also 4, as it refers to the same group of Slater determinants as $\tilde{g}_{\tilde{1}}$.

Taking the derivative of Eq. (12) with respect to $\mathtt{w}$ and noticing $M_I - M_{I-1} = g_I$, the excitation energy of the $I$th multiplet is obtained as

$$\omega_I = \frac{1}{g_I}\left[\left.\frac{dE^{\rm GOKII}_{I,\mathtt{w}}}{d\mathtt{w}'}\right|_{\mathtt{w}=\mathtt{w}_I} - \left.\frac{dE^{\rm GOKII}_{I-1,\mathtt{w}}}{d\mathtt{w}}\right|_{\mathtt{w}=\mathtt{w}_{I-1}}\right]. \tag{14}$$

Similar to the derivation for the GOK ensemble, we obtain

$$\begin{aligned} \frac{dE^{\rm GOKII}_{I,\mathtt{w}}}{d\mathtt{w}} =& \sum_{\mu=0}^{\infty}\left(\sum_{i=1}^{I}\sum_{k=1}^{g_i}\sum_{p=1}^{\tilde{g}_{\tilde{i}}}|C_{i,k,p}|^2 f_{\tilde{i},p,\mu}\right. \\ & \left. - \frac{M_I - g_0}{g_0}\sum_{k=1}^{g_1}\sum_{p=1}^{\tilde{g}_{\tilde{1}}}|C_{0,k,p}|^2 f_{\tilde{1},p,\mu}\right)\epsilon^I_\mu \\ & + \left.\frac{\partial E^{\rm GOKII}_{{\rm xc},I,\mathtt{w}}[n]}{\partial\mathtt{w}}\right|_{n=n^{\rm GOKII}_{I,\mathtt{w}}} \end{aligned} \tag{15}$$

where $f_{\tilde{i},p,\mu}$ is the occupation number of the $\mu$-th orbital in the $p$-th KS Slater determinant of the KS multiplet $\tilde{i}$. The $E^{\rm GOKII}_{\rm XC}$ in Eq. (15) is different from the $E_{\rm XC}$ in Eq. (8). Since there is an ambiguity in the definition of the ensemble Hartree energy [2], it is more general to replace the $E_{\rm XC}$ in Eq. (15) with $E_{\rm HXC}$. For notational simplicity, we still write $E_{\rm XC}$ in the main text.

Setting $\mathtt{w}_I = \mathtt{w}_{I-1} = 0$ in Eq. (14) allows us to express $\omega_I$ only in terms of ground-state properties ($\epsilon^I_\mu = \epsilon^{I-1}_\mu = \epsilon_\mu$, $n^{\rm GOKII}_{I,\mathtt{w}} = n^{\rm GOKII}_{I-1,\mathtt{w}} = n_0$, where $n_0$ is the ground-state density). Inserting Eq. (15) into Eq. (14) yields the DEC

$$\begin{aligned} \omega_I[n_0] = \omega^{\rm KS}_I[n_0] &+ \frac{1}{g_I}\left.\frac{\partial E^{\rm GOKII}_{{\rm xc},I,\mathtt{w}}[n]}{\partial\mathtt{w}}\right|_{n=n_0} \\ &- \frac{1}{g_I}\left.\frac{\partial E^{\rm GOKII}_{{\rm xc},I-1,\mathtt{w}}[n]}{\partial\mathtt{w}}\right|_{n=n_0}, \end{aligned} \tag{16}$$

as in the main text.

### DEC CALCULATION DETAILS

We calculate the excitation energy with the DEC, Eq. (16). The KS excitation frequency $\omega^{\rm KS}_I$ is known from the ground-state KS orbital energies. We only need to calculate $\partial E^{\rm GOKII}_{{\rm xc},i,\mathtt{w}}[n]/\partial\mathtt{w}\big|_{n=n^{\rm GOKII}_{i,\mathtt{w}}}$ for $i = I$ and $i = I-1$ at $\mathtt{w} = 0$. For simplicity, we omit $i$ from the expression in the following. We keep $\mathtt{w}$ in the expression instead of setting it to 0 to make the notation easier to follow. If we know the exact ensemble $E_{\rm XC}$, this partial derivative

(denoted as $G_{\mathtt{w}}$ in the following) can be calculated as [2]

$$\begin{aligned} G_{\mathtt{w}}[n_{\mathtt{w}}^{\mathrm{GOKII}}] &= \left.\frac{\partial E_{\mathrm{xc},\mathtt{w}}^{\mathrm{GOKII}}[n]}{\partial \mathtt{w}}\right|_{n=n_{\mathtt{w}}^{\mathrm{GOKII}}} \\ &= \frac{\partial E_{\mathrm{xc},\mathtt{w}}^{\mathrm{GOKII}}[n_{\mathtt{w}}^{\mathrm{GOKII}}]}{\partial \mathtt{w}} \\ &\quad - \int \mathrm{d}^3 r\, v_{\mathrm{xc},\mathtt{w}}^{\mathrm{GOKII}}[n_{\mathtt{w}}^{\mathrm{GOKII}}](\mathbf{r}) \frac{\partial n_{\mathtt{w}}^{\mathrm{GOKII}}(\mathbf{r})}{\partial \mathtt{w}}. \end{aligned} \tag{17}$$

Note that both the ensemble $E_{\mathrm{XC}}$ and the ensemble density depend on the weights parametrically. The ensemble $E_{\mathrm{XC}}$ is a functional of any trial density, not just defined at valid $n_{\mathtt{w}}^{\mathrm{GOKII}}$'s. Its derivative with respect to $\mathtt{w}$ cannot be taken directly as $\partial E_{\mathrm{xc},\mathtt{w}}^{\mathrm{GOKII}}[n_{\mathtt{w}}^{\mathrm{GOKII}}]/\partial\mathtt{w}$, so we have to subtract the contribution from the $\mathtt{w}$ dependence of the ensemble density, as shown in Eq. (17).

## Calculation details of DEC/SEHX

The functional form of SEHX for a general ensemble is given in Refs. [2, 3]:

$$\begin{aligned} E_{\mathrm{HX}}^{\mathrm{SEHX}} = \int \frac{\mathrm{d}^3 r \mathrm{d}^3 r'}{|\mathbf{r}-\mathbf{r}'|} \Bigg\{ &\sum_{\mu,\nu>\mu} \{ n_\mu^{\mathrm{orb}}(\mathbf{r}) n_\nu^{\mathrm{orb}}(\mathbf{r}') - \Re[n_\mu^{\mathrm{orb}}(\mathbf{r}',\mathbf{r}) n_\nu^{\mathrm{orb}}(\mathbf{r},\mathbf{r}')]\delta_{\sigma_\mu,\sigma_\nu} \} \sum_{i=0}^{I} \sum_{k=1}^{g_i} \mathtt{w}_{i,k} \sum_{p=1}^{\tilde{g}_{\tilde{i}}} |C_{i,k,p}|^2 f_{\tilde{i},p,\mu} f_{\tilde{i},p,\nu} \\ &+ \sum_{\substack{\mu,\nu>\mu \\ \kappa,\lambda>\kappa}} [\phi_\mu^*(\mathbf{r})\phi_\nu^*(\mathbf{r}')\phi_\kappa(\mathbf{r})\phi_\lambda(\mathbf{r}')\delta_{\sigma_\mu,\sigma_\kappa}\delta_{\sigma_\nu,\sigma_\lambda} - \phi_\mu^*(\mathbf{r})\phi_\nu^*(\mathbf{r}')\phi_\lambda(\mathbf{r})\phi_\kappa(\mathbf{r}')\delta_{\sigma_\mu,\sigma_\lambda}\delta_{\sigma_\nu,\sigma_\kappa}] \sum_{i=0}^{I} \sum_{k=1}^{g_i} \mathtt{w}_{i,k} \sum_{p,q\neq p}^{\tilde{g}_{\tilde{i}}} C_{i,k,p}^* C_{i,k,q} \\ &\times f_{\tilde{i},p,\mu} f_{\tilde{i},p,\nu} f_{\tilde{i},q,\kappa} f_{\tilde{i},q,\lambda} \prod_{\eta\neq\mu,\nu,\kappa,\lambda} \delta_{f_{\tilde{i},p,\eta}, f_{\tilde{i},q,\eta}} \Bigg\}, \end{aligned} \tag{18}$$

where $i$ denotes a multiplet; $k$ denotes a specific state in the $i$-th multiplet; $g_i$ is the degeneracy of the $i$-th multiplet; $\tilde{g}_{\tilde{i}}$ is the degeneracy of the corresponding Kohn-Sham (KS) multiplet; $p, q$ denote specific KS single Slater determinants; $\mu, \nu, \kappa, \lambda, \eta$ denote KS orbitals; $\mathtt{w}_{i,k}$ is the weight of the $k$-th state in the $i$-th multiplet; $C_{i,k,p}$ is the mixing coefficient of the $p$-th determinant to make up the $k$-th state in the $i$-th multiplet; $f_{\tilde{i},p,\mu}$ is the occupation number of the $\mu$-th orbital in the $p$-th determinant of the $\tilde{i}$-th KS multiplet; $\sigma$ denotes spin, $\phi$ denotes KS orbitals; $n_\mu^{\mathrm{orb}}(\mathbf{r}) = |\phi_\mu(\mathbf{r})|^2$ is the orbital density of the $\mu$-th orbital; and $n_\mu^{\mathrm{orb}}(\mathbf{r},\mathbf{r}') = \phi_\mu(\mathbf{r})\phi_\mu^*(\mathbf{r}')$.

SEHX as an orbital-dependent functional is an implicit functional of the density, and therefore we do not know its functional form for all trial densities. Eq. (17) is not applicable in DEC/SEHX calculations. If we differentiate Eq. (18) directly with respect to $\mathtt{w}$ [the $\mathtt{w}_{i,k}$ in Eq. (18) need to be replaced by the GOKII weights of Eq. (9) first], we would actually be calculating

$$\begin{aligned} \left.\frac{\partial E_{\mathrm{Hx},\mathtt{w}}^{\mathrm{GOKII}}[n_{\mathtt{w}}^{\mathrm{GOKII,KS}}[\{\phi_\mu\}]]}{\partial \mathtt{w}}\right|_{\phi_\mu=\phi_{\mu,\mathtt{w}}^{\mathrm{KS}}} &= \left.\frac{\partial E_{\mathrm{Hx},\mathtt{w}}^{\mathrm{GOKII}}[n]}{\partial \mathtt{w}}\right|_{n=n_{\mathtt{w}}^{\mathrm{GOKII,KS}}[\{\phi_{\mu,\mathtt{w}}^{\mathrm{KS}}\}]} \\ &\quad + \int \mathrm{d}^3 r \left[ \left.\frac{\delta E_{\mathrm{Hx},\mathtt{w}}^{\mathrm{GOKII}}[n]}{\delta n(\mathbf{r})}\right|_{n=n_{\mathtt{w}}^{\mathrm{GOKII,KS}}[\phi_{\mu,\mathtt{w}}^{\mathrm{KS}}]} \left.\frac{\partial n_{\mathtt{w}}^{\mathrm{GOKII,KS}}[\{\phi_\mu\}](\mathbf{r})}{\partial \mathtt{w}}\right|_{\phi_\mu=\phi_{\mu,\mathtt{w}}^{\mathrm{KS}}} \right]. \end{aligned} \tag{19}$$

This is the case because the KS orbitals are kept stationary when differentiating Eq. (18) directly. What we need for an DEC/SEHX calculation is $G_{\mathtt{w}}$, and that is actually the first term on the right hand side of Eq. (19) (which uses the KS ensemble density instead of the exact ensemble density). Therefore, for a DEC/SEHX calculation, we calculate $G_{\mathtt{w}}[n_{\mathtt{w}}]$ at $\mathtt{w}=0$ by

$$G_{\mathtt{w}=0}[n_{\mathtt{w}=0}] = \left.\frac{\partial E_{\mathrm{Hx},\mathtt{w}}[n_{\mathtt{w}}^{\mathrm{GOKII,KS}}[\{\phi_\mu\}]]}{\partial \mathtt{w}}\right|_{\phi_\mu=\phi_{\mu,\mathtt{w}=0}^{\mathrm{KS}}} - \int \mathrm{d}^3 r\, v_{\mathrm{HX}}[n_0^{\mathrm{KS}}](\mathbf{r}) \left.\frac{\partial n_{\mathtt{w}}^{\mathrm{GOKII,KS}}[\{\phi_\mu\}](\mathbf{r})}{\partial \mathtt{w}}\right|_{\phi_\mu=\phi_{\mu,\mathtt{w}=0}^{\mathrm{KS}}}, \tag{20}$$

i.e. the direct derivative of Eq. (18) minus a correction term. Inserting Eq. (20) into Eq. (16), we find that contributions from all the multiplets other than $i=0$ and $i=I$ cancel, and the summations over multiplets $i$ are simplified to sums of the $i=0$ and $i=I$ multiplets.

Here we show that with the GOKII ensemble, DEC/SEHX becomes effectively bi-ensemble. The elements of the $\mathbf{V}$ and $\mathbf{Q}_i$ matrices in the main text are

$$\begin{aligned} V_{\mu\nu\kappa\lambda}(\mathbf{r},\mathbf{r}') &= \frac{1}{2}\left[\phi^*_\mu(\mathbf{r})\phi^*_\nu(\mathbf{r}')\phi_\kappa(\mathbf{r})\phi_\lambda(\mathbf{r}')\delta_{\sigma_\mu,\sigma_\kappa}\delta_{\sigma_\nu,\sigma_\lambda} - \phi^*_\mu(\mathbf{r})\phi^*_\nu(\mathbf{r}')\phi_\lambda(\mathbf{r})\phi_\kappa(\mathbf{r}')\delta_{\sigma_\mu,\sigma_\lambda}\delta_{\sigma_\nu,\sigma_\kappa}\right], \\ Q_{i,\mu\nu\kappa\lambda} &= \sum_{k=1}^{g_i}\sum_{p,q=1}^{\tilde{g}_{\tilde{i}}} C^*_{i,k,p}C_{i,k,q} f_{\tilde{i},p,\mu} f_{\tilde{i},p,\nu} f_{\tilde{i},q,\kappa} f_{\tilde{i},q,\lambda} \prod_{\eta\neq\mu,\nu,\kappa,\lambda} \delta_{f_{\tilde{i},p,\eta},f_{\tilde{i},q,\eta}} \left\{\delta_{p,q}(\delta_{\mu,\kappa}\delta_{\nu,\lambda}-1)+1\right\}. \end{aligned} \tag{21}$$

Then the SEHX energy and its direct derivative with respect to $\mathtt{w}$ in the GOKII ensemble can be written as

$$\begin{aligned} E^{\text{SEHX,GOKII}}_{\text{Hx,I}} &= \frac{1}{2}\int \frac{\mathrm{d}^3r\mathrm{d}^3r'}{|\mathbf{r}-\mathbf{r}'|}\left[\frac{1-\mathtt{w}(M_I-g_0)}{g_0}\operatorname{tr}\{\mathbf{V}(\mathbf{r},\mathbf{r}')\cdot\mathbf{Q}_0\} + \mathtt{w}\sum_{i=1}^{I}\operatorname{tr}\{\mathbf{V}(\mathbf{r},\mathbf{r}')\cdot\mathbf{Q}_i\}\right], \\ \frac{dE^{\text{SEHX,GOKII}}_{Hx,I}[n^{GOKII,KS}_{\mathtt{w},I}]}{d\mathtt{w}} &= \frac{1}{2}\int \frac{\mathrm{d}^3r\mathrm{d}^3r'}{|\mathbf{r}-\mathbf{r}'|}\left[\frac{g_0-M_I}{g_0}\operatorname{tr}\{\mathbf{V}(\mathbf{r},\mathbf{r}')\cdot\mathbf{Q}_0\} + \sum_{i=1}^{I}\operatorname{tr}\{\mathbf{V}(\mathbf{r},\mathbf{r}')\cdot\mathbf{Q}_i\}\right]. \end{aligned} \tag{22}$$

The derivative of the GOKII KS ensemble density is

$$\frac{dn^{\text{GOKII,KS}}_{\mathtt{w},I}(\mathbf{r})}{d\mathtt{w}} = \frac{g_0-M_I}{g_0}n_{i=0}(\mathbf{r}) + \sum_{i=1}^{I} n_i(\mathbf{r}), \tag{23}$$

where $\tilde{n}_i = \sum_{k=1}^{g_0}\langle\Phi_{i,k}|\hat{n}(\mathbf{r})|\Phi_{i,k}\rangle$.

The bi-ensemble form is derived as the following:

$$\begin{aligned} \Delta\omega_I^{\text{DEC/SEHX}} &= \left.\frac{d}{d\mathtt{w}}\right|_{\mathtt{w}=0}\left(E^{\text{SEHX,GOKII}}_{\text{Hx,I}} - E^{\text{SEHX,GOKII}}_{\text{Hx,I-1}}\right) \\ &= \left.\left\{\frac{dE^{\text{SEHX,GOKII}}_{Hx,I}[n^{GOKII,KS}_{\mathtt{w},I}]}{d\mathtt{w}} - \frac{dE^{\text{SEHX,GOKII}}_{Hx,I-1}[n^{GOKII,KS}_{\mathtt{w},I-1}]}{d\mathtt{w}} - \int \mathrm{d}^3r\, v_{\text{HX}}(\mathbf{r})\left[\frac{dn^{\text{GOKII,KS}}_{\mathtt{w},I}(\mathbf{r})}{d\mathtt{w}} - \frac{dn^{\text{GOKII,KS}}_{\mathtt{w},I-1}(\mathbf{r})}{d\mathtt{w}}\right]\right\}\right|_{\mathtt{w}=0} \\ &= \frac{1}{2}\int\frac{\mathrm{d}^3r\mathrm{d}^3r'}{|\mathbf{r}-\mathbf{r}'|}\left[\frac{1}{g_I}\operatorname{tr}\{\mathbf{V}(\mathbf{r},\mathbf{r}')\cdot\mathbf{Q}_I\} - \frac{1}{g_0}\operatorname{tr}\{\mathbf{V}(\mathbf{r},\mathbf{r}')\cdot\mathbf{Q}_0\}\right] - \int \mathrm{d}^3r\, v_{\text{HX}}(\mathbf{r})\left[\frac{1}{g_I}\tilde{n}_I(\mathbf{r}) - \frac{1}{g_0}\tilde{n}_0(\mathbf{r})\right]. \end{aligned} \tag{24}$$

Eq. (24) is shown in the main text. Contributions from all the multiplets other than the ground state ($i=0$) and the excited state we want ($i=I$) cancel out. Eq. (24) is equivalent to evaluating the DEC Eq. (16) using SEHX with the above mentioned bi-ensemble.

As an example of Eq. (24), we apply it to the first and second excitations of the He atom. These excitations correspond to the $1s^2 \rightarrow 1s2s$ KS excitation. There are 4 KS Slater determinants for the 1s2s configuration:

$$\begin{aligned} \tilde{\Phi}_{\tilde{i}=1\text{ or }2,1}(\mathbf{r},\mathbf{r}') &\sim \hat{A}\phi_{1s\uparrow}(\mathbf{r})\phi_{2s\downarrow}(\mathbf{r}'), \\ \tilde{\Phi}_{\tilde{i}=1\text{ or }2,2}(\mathbf{r},\mathbf{r}') &\sim \hat{A}\phi_{1s\downarrow}(\mathbf{r})\phi_{2s\uparrow}(\mathbf{r}'), \\ \tilde{\Phi}_{\tilde{i}=1\text{ or }2,3}(\mathbf{r},\mathbf{r}') &\sim \hat{A}\phi_{1s\uparrow}(\mathbf{r})\phi_{2s\uparrow}(\mathbf{r}'), \\ \tilde{\Phi}_{\tilde{i}=1\text{ or }2,4}(\mathbf{r},\mathbf{r}') &\sim \hat{A}\phi_{1s\downarrow}(\mathbf{r})\phi_{2s\downarrow}(\mathbf{r}'), \end{aligned} \tag{25}$$

where $\hat{A}$ is the antisymmetrization operator. In the following, we label 1s↑ as orbital 1, 1s↓ as 2, 2s↑ as 3, 2s↓ as 4. The Slater determinants need to be combined into eigenstates of the total spin operator, and the linear combination coefficients are

$$\begin{aligned} &C_{1,1,1} = 1/\sqrt{2}, C_{1,1,2} = 1/\sqrt{2}, C_{1,1,3} = C_{1,1,4} = 0 \\ &C_{1,2,1} = C_{1,2,2} = 0, C_{1,2,3} = 1, C_{1,2,4} = 0 \\ &C_{1,3,1} = C_{1,3,2} = C_{1,3,3} = 0, C_{1,3,4} = 1 \\ &C_{2,1,1} = 1/\sqrt{2}, C_{2,1,2} = -1/\sqrt{2}, C_{2,1,3} = C_{2,1,4} = 0. \end{aligned} \tag{26}$$

Eq. (24) for the first excitation of the He atom is then

$$\begin{aligned}\Delta\omega_1^{\text{DEC/SEHX}} =&\frac{1}{2}\int \frac{\mathrm{d}^3r\mathrm{d}^3r'}{|\mathbf{r}-\mathbf{r}'|}\sum_{\mu,\nu,\kappa,\lambda=1}^{4} V_{\mu\nu\kappa\lambda}\left[\frac{1}{3}Q_{1,\mu\nu\kappa\lambda}-Q_{0,\mu\nu\kappa\lambda}\right] \\ &-\int \mathrm{d}^3r\; v_{\text{HX}}(\mathbf{r})[\frac{1}{3}n_{1,1}(\mathbf{r})+\frac{1}{3}n_{1,2}(\mathbf{r})+\frac{1}{3}n_{1,3}(\mathbf{r})-n_0(\mathbf{r})] \\ =&-(1|2)+1/3(1|3)+1/6(1|4)+1/6(2|3)+1/3(2|4)-1/6(14|23)'-1/6(23|14)' \\ &-\int \mathrm{d}^3r\; v_{\text{HX}}(\mathbf{r})[-1/2\,|\phi_1(\mathbf{r})|^2-1/2\,|\phi_2(\mathbf{r})|^2+1/2\,|\phi_3(\mathbf{r})|^2+1/2\,|\phi_4(\mathbf{r})|^2]\end{aligned} \tag{27}$$

where the notations

$$\begin{aligned}(\mu|\nu)&=\int \frac{\mathrm{d}^3r\mathrm{d}^3r'}{|\mathbf{r}-\mathbf{r}'|}\left[\phi_\mu^*(\mathbf{r})\phi_\nu^*(\mathbf{r}')\phi_\mu(\mathbf{r})\phi_\nu(\mathbf{r}')-\phi_\mu^*(\mathbf{r})\phi_\nu(\mathbf{r}')\phi_\nu(\mathbf{r})\phi_\mu(\mathbf{r}')\delta_{\sigma_\mu,\sigma_\nu}\right], \\ (\mu\nu|\kappa\lambda)'&=\int \frac{\mathrm{d}^3r\mathrm{d}^3r'}{|\mathbf{r}-\mathbf{r}'|}\phi_\mu^*(\mathbf{r})\phi_\nu^*(\mathbf{r}')\phi_\lambda(\mathbf{r})\phi_\kappa(\mathbf{r}')\delta_{\sigma_\mu,\sigma_\lambda}\delta_{\sigma_\nu,\sigma_\kappa}.\end{aligned} \tag{28}$$

For the second excitation of the He atom, we have

$$\begin{aligned}\Delta\omega_2^{\text{DEC/SEHX}} =&-(1|2)+1/2(1|4)+1/2(2|3)+1/2(14/23)'+1/2(23/14)' \\ &-\int \mathrm{d}^3r\; v_{\text{HX}}(\mathbf{r})[-1/2\,|\phi_1(\mathbf{r})|^2-1/2\,|\phi_2(\mathbf{r})|^2+1/2\,|\phi_3(\mathbf{r})|^2+1/2\,|\phi_4(\mathbf{r})|^2].\end{aligned} \tag{29}$$

## Calculation details of numerical DEC/exact

For systems where we can solve their exact densities, we can evaluate the derivatives required in the DEC Eq. (16) numerically: we can calculate the exact densities at $\mathtt{w}=0$ and $\mathtt{w}=\Delta$, where $\Delta$ is a small number, and then calculate the numerical derivative $(E^{\text{GOKII}}_{\text{xc},\mathtt{w}=\Delta}-E^{\text{GOKII}}_{\text{xc},\mathtt{w}=0})/\Delta$. However, this numerical derivative is not the $G_\mathtt{w}$ we want, because the density when taking the numerical derivative is not kept stationary (instead, we have $n^{\text{GOKII}}_{\mathtt{w}=\Delta}$ and $n^{\text{GOKII}}_{\mathtt{w}=0}$). When doing this numerical differentiation, we are actually calculating

$$\begin{aligned}\lim_{\Delta\to 0}\frac{E^{\text{GOKII}}_{\text{xc},\mathtt{w}=\Delta}-E^{\text{GOKII}}_{\text{xc},\mathtt{w}=0}}{\Delta}&=\frac{\partial E^{\text{GOKII}}_{\text{xc},\mathtt{w}}[n^{\text{GOKII}}_{\mathtt{w}}]}{\partial\mathtt{w}} \\ &=\left.\frac{\partial E^{\text{GOKII}}_{\text{xc},\mathtt{w}}[n]}{\partial\mathtt{w}}\right|_{n=n^{\text{GOKII}}_{\mathtt{w}}}+\int \mathrm{d}^3r\left[\left.\frac{\delta E^{\text{GOKII}}_{\text{xc},\mathtt{w}}[n]}{\delta n(\mathbf{r})}\right|_{n=n^{\text{GOKII}}_{\mathtt{w}}}\frac{\partial n^{\text{GOKII}}_{\mathtt{w}}(\mathbf{r})}{\partial\mathtt{w}}\right].\end{aligned} \tag{30}$$

The first term on the right hand side of Eq. (30) is the $G_\mathtt{w}$ we need. Therefore, for an DEC/exact calculation, we calculate $G_\mathtt{w}$ at $\mathtt{w}=0$ by

$$G_{\mathtt{w}=0}[n^{\text{GOKII}}_{\mathtt{w}=0}]\approx\frac{E^{\text{GOKII}}_{\text{xc},\mathtt{w}=\Delta}-E^{\text{GOKII}}_{\text{xc},\mathtt{w}=0}}{\Delta}-\int \mathrm{d}^3r\; v_{\text{XC}}[n_0](\mathbf{r})\frac{n^{\text{GOKII}}_{\mathtt{w}=\Delta}(\mathbf{r})-n_0(\mathbf{r})}{\Delta}. \tag{31}$$

We use $\Delta=0.0001$ for the 1D two-electron contact-interaction Hooke's atom in main text.

## THE INFLUENCE OF THE ERRORS IN KS POTENTIALS

The exact KS potential and orbitals of He and Be atoms are used in DEC/SEHX and TDDFT/ALDA calculations, which eliminated the errors in the KS potentials. Here we show the size of such errors in He and Be atoms. We use the KLI [4] approximation of the exact exchange functional (denoted as EXX/KLI in the following) to calculate the approximated ground-state KS potential and orbitals, and use these in DEC/SEHX and TDDFT/ALDA calculations. The results are plotted in Figs. 1 and 2. The accuracy of DEC/SEHX is also higher than TDDFT/ALDA here, but the absolute error is much bigger than in the main text, which is due to the error in the approximated ground-state KS orbital energies, induced by the non-exact ground-state density.

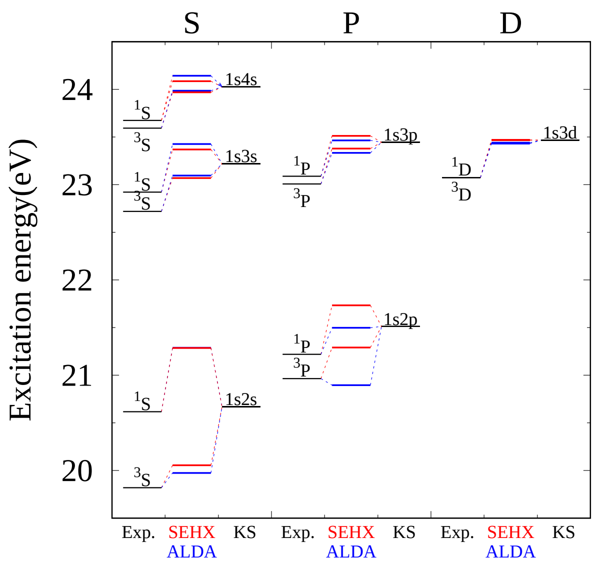


FIG. 1. Same as Fig. 1 of main text, except based on the EXX/KLI ground state.

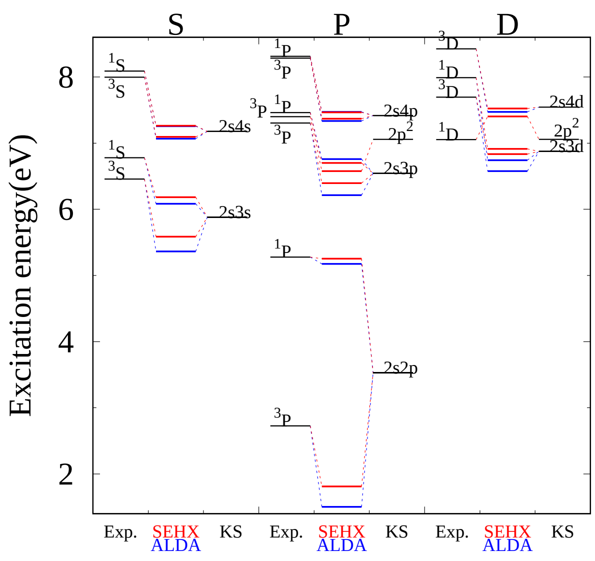


FIG. 2. Same as Fig. 2 of main text, except based on the EXX/KLI ground state.

## CALCULATION RESULTS OF OTHER ATOMS AND IONS BASED ON THE EXX/KLI GROUND STATE

Here we provide DEC/SEHX calculation results of other atoms and ions.

Since the exact KS potentials of these systems are unavailable to us, these calculations are carried out using EXX/KLI potentials and orbitals. For the $Li^+$ ion, Mg atom and Ca atom, we also included TDDFT/ALDA results, and we find that in most of the cases DEC/SEHX performs better than TDDFT/ALDA. For Li, Na, K atoms, the KS excitation energies are quite far from the experimental excitation energies (several eV apart), but DEC/SEHX can still yield accurate results. For B and Al atoms, there are KS states that do not have the same ordering as in the real system, but DEC/SEHX can correct the ordering for states with the same angular momentum (but not global ordering).

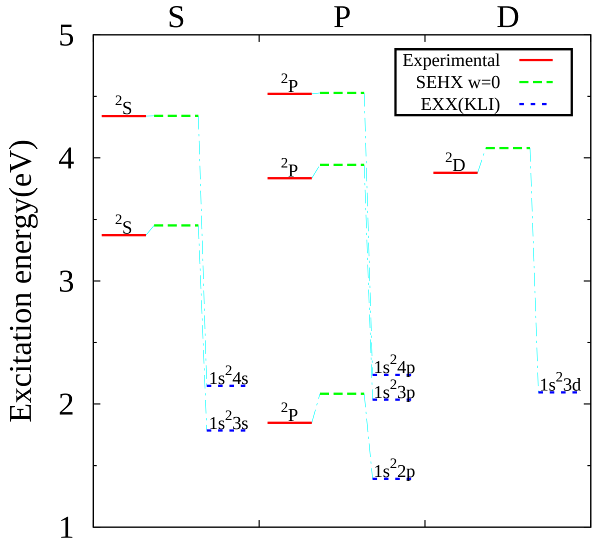


FIG. 3. Same as Fig. 1, except for the Li atom[5, 6]. A spin-restricted ground state is used to satisfy the symmetry requirement of SEHX.

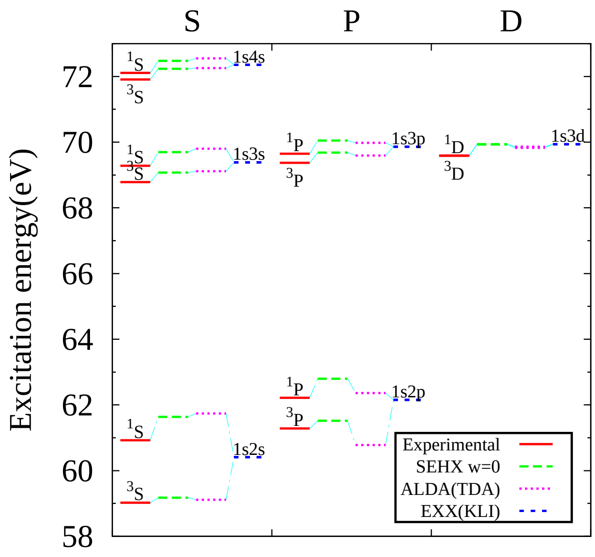


FIG. 4. Same as Fig. 1, except for the $Li^+$ ion[5, 6].

| Atom/Ion | He(EX) | Be(EX) | He | Be | Li | Li$^+$ | B | Na | Mg | Al | K | Ca |
|---|---|---|---|---|---|---|---|---|---|---|---|---|
| Figure | | | 1 | 2 | 3 | 4 | 5 | 6 | 7 | 8 | 9 | 10 |
| Table | II | III | IV | V | VI | VII | VIII | IX | X | XI | XII | XIII |

TABLE I. Table of contents for the calculation results. EX denotes results using the exact KS ground state, while all other calculations use the EXX ground state.

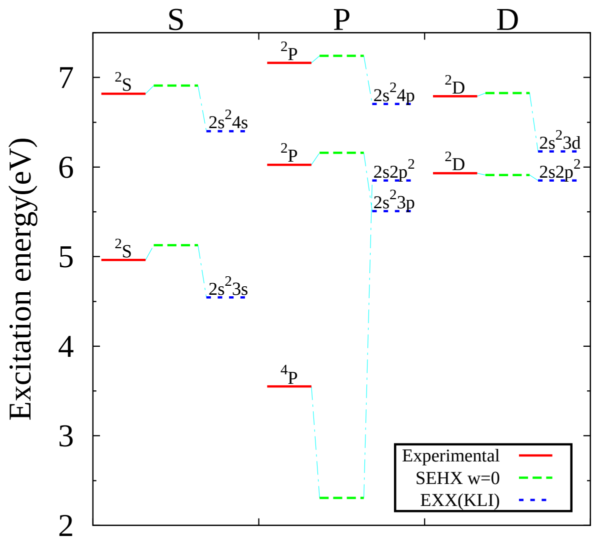


FIG. 5. Same as Fig. 3, except for the B atom[5, 7].

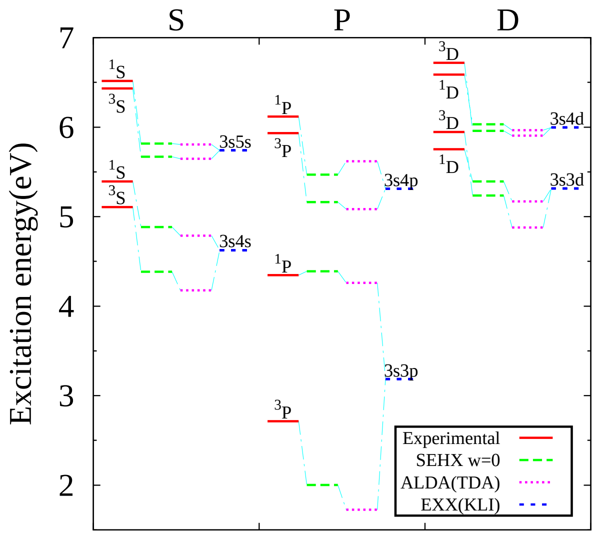


FIG. 7. Same as Fig. 1, except for the Mg atom[5, 9].

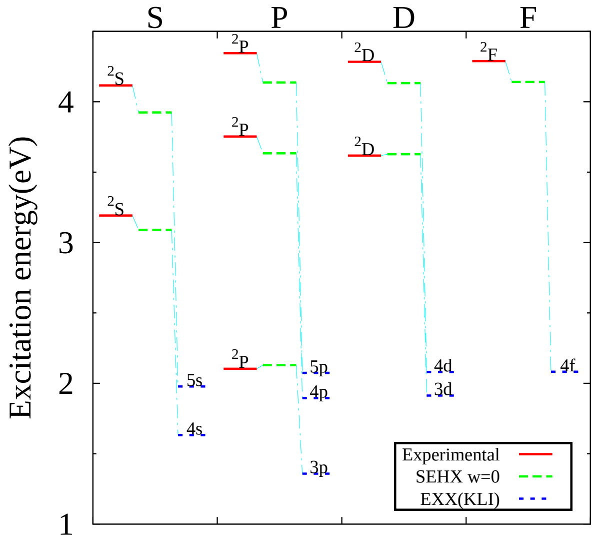


FIG. 6. Same as Fig. 3, except for the Na atom[5, 8].

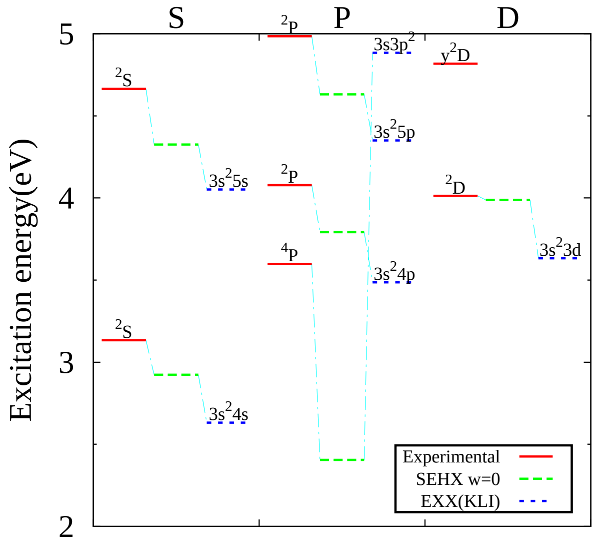


FIG. 8. Same as Fig. 3, except for the Al atom[5, 10].


[1] E. K. U. Gross, L. N. Oliveira, and W. Kohn. Density-functional theory for ensembles of fractionally occupied states. I. Basic formalism. *Phys. Rev. A*, 37:2809, 1988.

[2] A. Pribram-Jones, Z.-H. Yang, J. R. Trail, K. Burke, R. J. Needs, and C. A. Ullrich. Excitations and benchmark ensemble density functional theory for two electrons. *J. Chem. Phys.*, 140:18A541, 2014.

[3] Z.-H. Yang, J. R. Trail, A. Pribram-Jones, K. Burke, R. J. Needs, and C. A. Ullrich. Exact and approximate

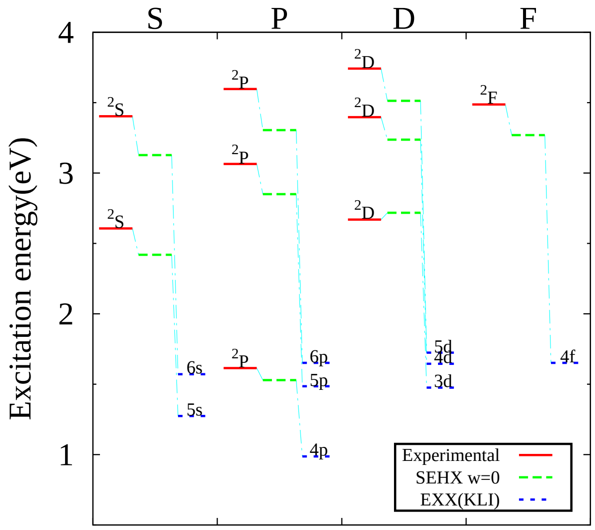


FIG. 9. Same as Fig. 3, except for the K atom[5, 11–15].

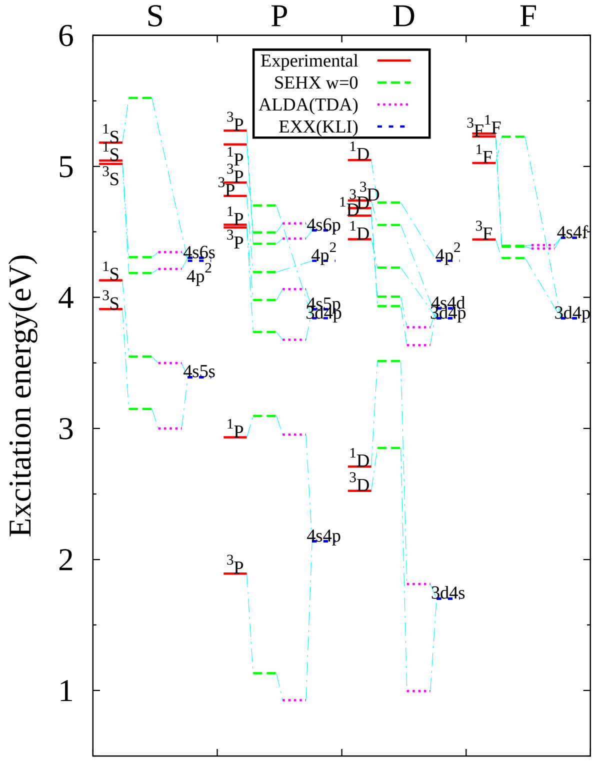


FIG. 10. Same as Fig. 1, except for the Ca atom[5, 11].

| Conf. | Term | Exp. | DEC SEHX | exact KS | TDDFT ALDA |
|---|---|---|---|---|---|
| 1s2s | $^3$S | 19.82 | 19.68 | 20.30 | 19.60 |
| 1s2s | $^1$S | 20.62 | 20.92 | 20.30 | 20.92 |
| 1s2p | $^3$P | 20.96 | 20.94 | 21.15 | 20.55 |
| 1s2p | $^1$P | 21.22 | 21.36 | 21.15 | 21.13 |
| 1s3s | $^3$S | 22.72 | 22.69 | 22.84 | 22.71 |
| 1s3s | $^1$S | 22.92 | 22.99 | 22.84 | 23.05 |
| 1s3p | $^3$P | 23.007 | 23.004 | 23.068 | 22.957 |
| 1s3d | $^3$D | 23.0736 | 23.0813 | 23.0825 | 23.0468 |
| 1s3d | $^1$D | 23.0741 | 23.0836 | 23.0825 | 23.0568 |
| 1s3p | $^1$P | 23.087 | 23.133 | 23.068 | 23.086 |
| 1s4s | $^3$S | 23.594 | 23.586 | 23.645 | 23.603 |
| 1s4s | $^1$S | 23.674 | 23.704 | 23.645 | 23.764 |

| n | MAE DEC/SEHX | MAE TDDFT/ALDA |
|---|---|---|
| 2 | 0.15 | 0.26 |
| 3 | 0.03 | 0.04 |
| 4 | 0.02 | 0.05 |
| All | 0.07 | 0.11 |

TABLE II. Excitation energy data for the He atom calculated with the exact KS ground state (Fig. 1 of the main text). All energies are in eV. The mean absolute error (MAE) of $\Delta\omega_I$ are also listed, where the excitations are grouped by the principal quantum number $n$ of the excited KS electron.

kohn-sham potentials in ensemble density-functional theory. *Phys. Rev. A*, 90:042501, 2014.

[4] J. B. Krieger, Y. Li, and G. J. Iafrate. *Phys. Rev. A*, 45:101, 1992.

[5] http://www.nist.gov/pml/data/asd.cfm.

[6] C. E. Moore. Atomic energy levels as derived from the analysis of optical spectra c hydrogen through vanadium. In *Nat. Stand. Ref. Data Ser., NSRDS-NBS 35 Vol. I.* Nat. Bur. Stand., 1971.

[7] A. E. Kramida and A. N. Ryabtsev. A critical compilation of energy levels and spectral lines of neutral boron. *Phys. Scr.*, 76:544, 2007.

[8] J. E. Sansonetti. Wavelengths, transition probabilities, and energy levels for the spectra of sodium (Na I—Na XI). *J. Phys. Chem. Ref. Data*, 37:1659, 2008.

[9] W. C. Martin and R. Zalubas. Energy levels of magnesium, Mg I through Mg XII. *J. Phys. Chem. Ref. Data*, 9:1, 1980.

[10] W. C. Martin and R. Zalubas. Energy levels of aluminum, Al I through Al XIII. *J. Phys. Chem. Ref. Data*, 8:817, 1979.

[11] J. Sugar and C. Corliss. Atomic energy levels of the iron-period elements: Potassium through nickel. *J. Phys. Chem. Ref. Data*, 14(Suppl. 2):1, 1985.

[12] S. Falke, E. Tiemann, C. Lisdat, H. Schnatz, and G. Grosche. Transition frequencies of the d lines of $^{39}$K, $^{40}$K, and $^{41}$K measured with a femtosecond laser frequency comb. *Phys. Rev. A*, 74:032503, 2006.

[13] I. Johansson and N. Svendenius. An intensity problem in the spectrum of potassium. *Phys. Scr.*, 5:129, 1972.

[14] D. C. Thompson, M. S. O'Sullivan, B. P. Stoicheff, and G. X. Xu. Doppler-free two-photon absorption spectrum of potassium. *Can. J. Phys.*, 61:949, 1983.

[15] P. Risberg. A revision of the term systems for Na I and K I based on hollow-cathode observation. *Ark. Fys. (Stockholm)*, 10:583, 1956.

| Conf. | Term | Exp. | DEC | TDDFT | exact |
|---|---|---|---|---|---|
| | | | SEHX | ALDA | KS |
| 2s2p | $^3$P | 2.72 | 1.69 | 1.45 | 3.58 |
| 2s2p | $^1$P | 5.28 | 5.39 | 5.47 | 3.58 |
| 2s3s | $^3$S | 6.46 | 6.34 | 6.10 | 6.63 |
| 2s3s | $^1$S | 6.78 | 6.95 | 6.84 | 6.63 |
| 2p$^2$ | $^1$D | 7.05 | 7.34 | N/A | 7.17 |
| 2s3p | $^3$P | 7.303 | 7.174 | 6.955 | 7.304 |
| 2p$^2$ | $^3$P | 7.40 | 6.44 | N/A | 7.17 |
| 2s3p | $^1$P | 7.462 | 7.448 | 7.425 | 7.304 |
| 2s3d | $^3$D | 7.69 | 7.65 | 7.34 | 7.68 |
| 2s3d | $^1$D | 7.99 | 7.75 | 7.54 | 7.68 |
| 2s4s | $^3$S | 8.00 | 7.96 | 7.92 | 8.03 |
| 2s4s | $^1$S | 8.09 | 8.13 | 8.11 | 8.03 |
| 2s4p | $^3$P | 8.28 | 8.23 | 8.18 | 8.26 |
| 2s4p | $^1$P | 8.31 | 8.32 | 8.29 | 8.26 |
| 2s4d | $^3$D | 8.424 | 8.396 | 8.324 | 8.404 |

| n | MAE | MAE |
|---|---|---|
| | DEC/SEHX | TDDFT/ALDA |
| 2 | 0.60 | 0.73 |
| 3 | 0.12 | 0.27 |
| 4 | 0.03 | 0.06 |
| All | 0.22 | 0.26 |

TABLE III. Excitation energy data for the Be atom calculated with the exact KS ground state (Fig. 2 of the main text). All energies are in eV.

| Conf. | Term | Exp. | DEC | TDDFT | EXX |
|---|---|---|---|---|---|
| | | | SEHX | ALDA | KS |
| 2s2p | $^3$P | 2.72 | 1.81 | 1.50 | 3.53 |
| 2s2p | $^1$P | 5.28 | 5.25 | 5.18 | 3.53 |
| 2s3s | $^3$S | 6.46 | 5.59 | 5.36 | 5.88 |
| 2s3s | $^1$S | 6.78 | 6.18 | 6.08 | 5.88 |
| 2p$^2$ | $^1$D | 7.05 | 7.40 | N/A | 7.06 |
| 2s3p | $^3$P | 7.30 | 6.40 | 6.21 | 6.54 |
| 2p$^2$ | $^3$P | 7.40 | 6.58 | N/A | 7.06 |
| 2s3p | $^1$P | 7.46 | 6.70 | 6.76 | 6.54 |
| 2s3d | $^3$D | 7.694 | 6.835 | 6.577 | 6.875 |
| 2s3d | $^1$D | 7.988 | 6.915 | 6.743 | 6.875 |
| 2s4s | $^3$S | 7.998 | 7.093 | 7.068 | 7.177 |
| 2s4s | $^1$S | 8.089 | 7.264 | 7.256 | 7.177 |
| 2s4p | $^3$P | 8.284 | 7.368 | 7.336 | 7.416 |
| 2s4p | $^1$P | 8.311 | 7.467 | 7.473 | 7.416 |
| 2s4d | $^3$D | 8.424 | 7.524 | 7.471 | 7.544 |

| n | MAE | MAE |
|---|---|---|
| | DEC/SEHX | TDDFT/ALDA |
| 2 | 0.53 | 0.66 |
| 3 | 0.84 | 0.99 |
| 4 | 0.88 | 0.90 |
| All | 0.77 | 0.90 |

TABLE V. Excitation energy data for the Be atom calculated with the EXX ground state (Fig. 2). All energies are in eV.

| Conf. | Term | Exp. | DEC | EXX | TDDFT |
|---|---|---|---|---|---|
| | | | SEHX | KS | ALDA |
| 1s2s | $^3$S | 19.82 | 20.06 | 20.67 | 19.97 |
| 1s2s | $^1$S | 20.62 | 21.28 | 20.67 | 21.29 |
| 1s2p | $^3$P | 20.96 | 21.29 | 21.51 | 20.90 |
| 1s2p | $^1$P | 21.22 | 21.73 | 21.51 | 21.50 |
| 1s3s | $^3$S | 22.72 | 23.07 | 23.22 | 23.09 |
| 1s3s | $^1$S | 22.92 | 23.37 | 23.22 | 23.43 |
| 1s3p | $^3$P | 23.01 | 23.38 | 23.44 | 23.33 |
| 1s3d | $^3$D | 23.0736 | 23.4655 | 23.4665 | 23.4315 |
| 1s3d | $^1$D | 23.0741 | 23.4679 | 23.4665 | 23.4413 |
| 1s3p | $^1$P | 23.09 | 23.51 | 23.44 | 23.46 |
| 1s4s | $^3$S | 23.59 | 23.97 | 24.03 | 23.98 |
| 1s4s | $^1$S | 23.67 | 24.08 | 24.03 | 24.14 |

| n | MAE | MAE |
|---|---|---|
| | DEC/SEHX | TDDFT/ALDA |
| 2 | 0.44 | 0.29 |
| 3 | 0.40 | 0.38 |
| 4 | 0.40 | 0.43 |
| All | 0.41 | 0.36 |

TABLE IV. Excitation energy data for the He atom calculated with the EXX ground state (Fig. 1). All energies are in eV.

| Conf. | Term | Exp. | DEC | EXX |
|---|---|---|---|---|
| | | | SEHX | KS |
| 2p | $^2$P | 1.85 | 2.08 | 1.39 |
| 3s | $^2$S | 3.37 | 3.45 | 1.78 |
| 3p | $^2$P | 3.83 | 3.94 | 2.04 |
| 3d | $^2$D | 3.88 | 4.08 | 2.09 |
| 4s | $^2$S | 4.34 | 4.34 | 2.15 |
| 4p | $^2$P | 4.52 | 4.53 | 2.24 |

| n | MAE |
|---|---|
| | DEC/SEHX |
| 2 | 0.23 |
| 3 | 0.13 |
| 4 | 0.005 |
| All | 0.10 |

TABLE VI. Excitation energy data for the Li atom calculated with the EXX ground state (Fig. 3). All energies are in eV.

| Conf. | Term | Exp. | DEC SEHX | TDDFT ALDA | EXX KS |
|---|---|---|---|---|---|
| 1s2s | $^3$S | 59.02 | 59.17 | 59.11 | 60.40 |
| 1s2s | $^1$S | 60.92 | 61.64 | 61.74 | 60.40 |
| 1s2p | $^3$P | 61.28 | 61.51 | 60.78 | 62.16 |
| 1s2p | $^1$P | 62.22 | 62.80 | 62.36 | 62.16 |
| 1s3s | $^3$S | 68.78 | 69.07 | 69.11 | 69.38 |
| 1s3s | $^1$S | 69.28 | 69.69 | 69.80 | 69.38 |
| 1s3p | $^3$P | 69.37 | 69.68 | 69.59 | 69.86 |
| 1s3d | $^3$D | 69.58 | 69.93 | 69.82 | 69.93 |
| 1s3d | $^1$D | 69.59 | 69.94 | 69.86 | 69.93 |
| 1s3p | $^1$P | 69.65 | 70.05 | 69.98 | 69.86 |
| 1s4s | $^3$S | 71.91 | 72.23 | 72.26 | 72.35 |
| 1s4s | $^1$S | 72.11 | 72.48 | 72.55 | 72.35 |

| n | MAE DEC/SEHX | MAE TDDFT/ALDA |
|---|---|---|
| 2 | 0.42 | 0.39 |
| 3 | 0.35 | 0.32 |
| 4 | 0.34 | 0.40 |
| All | 0.37 | 0.35 |

TABLE VII. Excitation energy data for the $Li^+$ ion calculated with the EXX ground state (Fig. 4). All energies are in eV.

| Conf. | Term | Exp. | DEC SEHX | EXX KS |
|---|---|---|---|---|
| 2s2p$^2$ | $^4$P | 3.55 | 2.31 | 5.85 |
| 2s$^2$3s | $^2$S | 4.96 | 5.13 | 4.54 |
| 2s2p$^2$ | $^2$D | 5.93 | 5.91 | 5.85 |
| 2s$^2$3p | $^2$P | 6.02 | 6.16 | 5.51 |
| 2s$^2$3d | $^2$D | 6.79 | 6.83 | 6.17 |
| 2s$^2$4s | $^2$S | 6.82 | 6.91 | 6.40 |
| 2s$^2$4p | $^2$P | 7.16 | 7.24 | 6.70 |

| n | MAE DEC/SEHX |
|---|---|
| 2 | 0.63 |
| 3 | 0.12 |
| 4 | 0.08 |
| All | 0.25 |

TABLE VIII. Excitation energy data for the B atom calculated with the EXX ground state (Fig. 5). All energies are in eV.

| Conf. | Term | Exp. | DEC SEHX | EXX KS |
|---|---|---|---|---|
| 3p | $^2$P | 2.10 | 2.13 | 1.36 |
| 4s | $^2$S | 3.19 | 3.09 | 1.63 |
| 3d | $^2$D | 3.617 | 3.628 | 1.913 |
| 4p | $^2$P | 3.753 | 3.634 | 1.895 |
| 5s | $^2$S | 4.12 | 3.92 | 1.98 |
| 4d | $^2$D | 4.2835 | 4.1316 | 2.0800 |
| 4f | $^2$F | 4.2882 | 4.1397 | 2.0817 |
| 5p | $^2$P | 4.3446 | 4.1378 | 2.0734 |

| n | MAE DEC/SEHX |
|---|---|
| 3 | 0.02 |
| 4 | 0.13 |
| 5 | 0.20 |
| All | 0.12 |

TABLE IX. Excitation energy data for the Na atom calculated with the EXX ground state (Fig. 6). All energies are in eV.

| Conf. | Term | Exp. | DEC SEHX | TDDFT ALDA | EXX KS KS |
|---|---|---|---|---|---|
| 3s3p | $^3$P | 2.71 | 2.00 | 1.72 | 3.18 |
| 3s3p | $^1$P | 4.34 | 4.39 | 4.26 | 3.18 |
| 3s4s | $^3$S | 5.11 | 4.38 | 4.18 | 4.63 |
| 3s4s | $^1$S | 5.39 | 4.88 | 4.79 | 4.63 |
| 3s3d | $^1$D | 5.753 | 5.393 | 5.171 | 5.315 |
| 3s4p | $^3$P | 5.932 | 5.163 | 5.083 | 5.312 |
| 3s3d | $^3$D | 5.946 | 5.236 | 4.878 | 5.315 |
| 3s4p | $^1$P | 6.12 | 5.47 | 5.62 | 5.31 |
| 3s5s | $^3$S | 6.43 | 5.67 | 5.65 | 5.74 |
| 3s5s | $^1$S | 6.52 | 5.82 | 5.81 | 5.74 |
| 3s4d | $^1$D | 6.59 | 6.03 | 5.96 | 6.00 |
| 3s4d | $^3$D | 6.72 | 5.96 | 5.90 | 6.00 |

| n | MAE DEC/SEHX | MAE TDDFT/ALDA |
|---|---|---|
| 3 | 0.46 | 0.68 |
| 4 | 0.66 | 0.72 |
| 5 | 0.73 | 0.74 |
| All | 0.60 | 0.71 |

TABLE X. Excitation energy data for the Mg atom calculated with the EXX ground state (Fig. 7). All energies are in eV.

| Conf. | Term | Exp. | DEC SEHX | EXX KS |
|---|---|---|---|---|
| $3s^24s$ | $^2S$ | 3.13 | 2.92 | 2.63 |
| $3s3p^2$ | $^4P$ | 3.60 | 2.40 | 4.88 |
| $3s^23d$ | $^2D$ | 4.01 | 3.99 | 3.63 |
| $3s^24p$ | $^2P$ | 4.08 | 3.79 | 3.48 |
| $3s^25s$ | $^2S$ | 4.66 | 4.32 | 4.05 |
| $3s^2nd$ | $y^2D$ | 4.82 | N/A | N/A |
| $3s^25p$ | $^2P$ | 4.98 | 4.63 | 4.35 |
| n | | MAE DEC/SEHX | | |
| 3 | | 0.61 | | |
| 4 | | 0.25 | | |
| 5 | | 0.34 | | |
| All | | 0.40 | | |

TABLE XI. Excitation energy data for the Al atom calculated with the EXX ground state (Fig. 8). All energies are in eV.

| Conf. | Term | Exp. | DEC SEHX | EXX KS |
|---|---|---|---|---|
| 4p | $^2P$ | 1.61 | 1.53 | 0.99 |
| 5s | $^2S$ | 2.61 | 2.42 | 1.27 |
| 3d | $^2D$ | 2.67 | 2.72 | 1.48 |
| 5p | $^2P$ | 3.06 | 2.85 | 1.48 |
| 4d | $^2D$ | 3.397 | 3.238 | 1.646 |
| 6s | $^2S$ | 3.403 | 3.127 | 1.572 |
| 4f | $^2F$ | 3.487 | 3.269 | 1.651 |
| 6p | $^2P$ | 3.596 | 3.304 | 1.652 |
| 5d | $^2D$ | 3.74 | 3.51 | 1.72 |
| n | | MAE DEC/SEHX | | |
| 4 | | 0.15 | | |
| 5 | | 0.21 | | |
| 6 | | 0.28 | | |
| All | | 0.19 | | |

TABLE XII. Excitation energy data for the K atom calculated with the EXX ground state (Fig. 9). All energies are in eV.

| Conf. | Term | Exp. | DEC SEHX | TDDFT ALDA | EXX KS |
|---|---|---|---|---|---|
| 4s4p | $^3P$ | 1.89 | 1.13 | 0.92 | 2.14 |
| 3d4s | $^3D$ | 2.52 | 2.85 | 1.00 | 1.70 |
| 3d4s | $^1D$ | 2.71 | 3.51 | 1.81 | 1.70 |
| 4s4p | $^1P$ | 2.93 | 3.10 | 2.95 | 2.14 |
| 4s5s | $^3S$ | 3.91 | 3.15 | 3.00 | 3.39 |
| 4s5s | $^1S$ | 4.13 | 3.55 | 3.50 | 3.39 |
| 3d4p | $^3F$ | 4.442 | 4.300 | N/A | 3.840 |
| 3d4p | $^1D$ | 4.443 | 4.227 | N/A | 3.840 |
| 4s5p | $^3P$ | 4.53 | 3.74 | 3.68 | 3.91 |
| 4s5p | $^1P$ | 4.55 | 3.98 | 4.06 | 3.91 |
| 4s4d | $^1D$ | 4.62 | 4.00 | 3.77 | 3.92 |
| 4s4d | $^3D$ | 4.68 | 3.93 | 3.64 | 3.92 |
| 3d4p | $^3D$ | 4.74 | 4.55 | N/A | 3.84 |
| $4p^2$ | $^3P$ | 4.77 | 4.19 | N/A | 4.28 |
| 3d4p | $^3P$ | 4.88 | 4.70 | N/A | 3.84 |
| 4s6s | $^3S$ | 5.02 | 4.18 | 4.22 | 4.30 |
| 3d4p | $^1F$ | 5.03 | 5.23 | N/A | 3.84 |
| 4s6s | $^1S$ | 5.045 | 4.306 | 4.345 | 4.301 |
| $4p^2$ | $^1D$ | 5.049 | 4.724 | N/A | 4.279 |
| 4s6p | $^1P$ | 5.17 | 4.50 | 4.56 | 4.51 |
| $4p^2$ | $^1S$ | 5.18 | 5.52 | N/A | 4.28 |
| 4s4f | $^3F$ | 5.23 | 4.38 | 4.37 | 4.46 |
| 4s4f | $^1F$ | 5.25 | 4.39 | 4.40 | 4.46 |
| 4s6p | $^3P$ | 5.27 | 4.41 | 4.45 | 4.52 |
| n | | MAE DEC/SEHX | | MAE TDDFT/ALDA | |
| 3 | | 0.29 | | 1.21 | |
| 4 | | 0.58 | | 0.76 | |
| 5 | | 0.68 | | 0.72 | |
| 6 | | 0.78 | | 0.73 | |
| All | | 0.55 | | 0.80 | |

TABLE XIII. Excitation energy data for the Ca atom calculated with the EXX ground state (Fig. 10). All energies are in eV.
